# Supplementary material for: MARVEL-40M+: Multi-Level Visual Elaboration for High-Fidelity Text-to-3D Content Creation
Source: arXiv:2411.17945 source file (2025-03-26)
Supplement: Supplementary file 1 [file 0_test.tex]

% \begin{table}[h!]
%     \centering
%     \resizebox{\columnwidth}{!}{%
%     \begin{tabular}{llcccccc}
%         \toprule
%         & Finetune & \multirow{2}{*}{FID $\downarrow$} & CLIP & \multicolumn{4}{c}{CLIP R-Precision (2k)} \\
%         \cmidrule(lr){5-8}
%         & Dataset & & Score & R@1 & R@5 & R@10 \\
%         \midrule
%         \multirow{4}{*}{\rotatebox[origin=c]{-270}{Point-E}} & Pretrained & 36.1 & 72.4 & 6.0 & 16.2 & 22.4 \\
%         & 30k (Human) & 34.6 & 74.4 & 8.2 & 21.3 & 29.1 \\
%         & 30k (Cap3D~\cite{cap3d}) & 33.7 & 75.0 & 10.4 & 24.3 & 32.1 \\
%         & 350k (Cap3D~\cite{cap3d}) & 32.8 & 75.6 & 12.4 & 28.1 & 36.9 \\
%         & 360k (3DTopia~\cite{3dtopia}) &  &  &  &  &  \\
%          & 660k (Cap3D~\cite{cap3d}) &  &  &  &  &  \\
%           & 660k (MARVEL) &  &  &  &  &  \\
%         \midrule
%         \multirow{4}{*}{\rotatebox[origin=c]{-270}{Shap-E}} & Pretrained & 37.2 & 80.4 & 20.3 & 39.7 & 48.7 \\
%         & 30k (Human) & 36.0 & 79.6 & 18.6 & 36.3 & 45.3 \\
%         & 30k (Cap3D~\cite{cap3d}) & 37.2 & 79.4 & 19.1 & 37.5 & 46.1 \\
%         & 350k (Cap3D~\cite{cap3d}) & 35.5 & 79.1 & 20.0 & 38.8 & 47.3 \\
%          & 360k (3DTopia~\cite{3dtopia}) &  &  &  &  &  \\
%         & 660k (Cap3D~\cite{cap3d}) & & & & & \\
%         & 660k (MARVEL) & \textbf{34.4} &  &  &  &  \\
%         \bottomrule
%     \end{tabular}
%     }
%     \caption{Comparison of FID, CLIP Score, and CLIP R-Precision for Point-E and Shap-E models across various finetune datasets. (Will be in supplementary)}
% \end{table}

\section{\textcolor{red}{Supplementary Material}}

\subsection{TODO LIST}

\begin{enumerate}
    \item An entire section about Data statistics. Density plot of words per caption. CAP3D - Figure 3 right image.
    \item Word cloud
    \item More annotation results for Objaverse -  sorted by categories/domains.
    \item More annotations of ShapeNet, ABO, Pix3D, Toys4K, GSO, Omniobject3D.
    \item More Baseline results - Comparative (50 random samples)
    \item More Baseline Results - 
\end{enumerate}

\subsection*{Semantic Compression Score (SCS)}\label{Metric: SCS}

The \textit{Semantic Compression Score (SCS)} is a metric designed to evaluate the balance between semantic retention and text compression across different levels of summarization. Let \( l_i \) and \( l_j \) represent two levels in the compression hierarchy, where \( j > i \) indicates that \( l_j \) is a more compressed version of \( l_i \). The metric combines two key components:

\begin{itemize}
    \item \textbf{Semantic Similarity (\( s \))}: This measures the degree of semantic information retention between \( l_i \) and \( l_j \). It is defined as:
    \begin{equation}
        s = \text{cosine\_similarity}(\text{embedding}(l_i), \text{embedding}(l_j)),
    \end{equation}
    where \( 0 \leq s \leq 1 \), with 0 indicating no semantic similarity and 1 indicating perfect retention.

    \item \textbf{Compression Ratio (\( c \))}: This represents the proportion of text reduction from \( l_i \) to \( l_j \) and is defined as:
    \begin{equation}
        c = 1 - \frac{\text{word count of } l_j}{\text{word count of } l_i},
    \end{equation}
    where \( 0 \leq c \leq 1 \), with 0 indicating no compression and 1 indicating maximum compression (i.e., \( l_j \) approaches zero length).
\end{itemize}

The \textit{Semantic Compression Score (SCS)} is calculated as the harmonic mean of \( s \) and \( c \):
\begin{equation}
    \text{SCS} = \frac{2 \cdot s \cdot c}{s + c},
\end{equation}
ensuring a bounded score between 0 and 1. This metric emphasizes balance by penalizing cases where one of the components is disproportionately low, providing a comprehensive measure of how well semantic information is preserved while achieving effective compression. An SCS close to 1 indicates an optimal balance with high semantic retention and significant compression, while lower scores suggest potential information loss or insufficient compression.

Sematic similarity~\cite{reimers2019sentence} and compression ratio~\cite{compression_ratio}.
